# Supplementary material for: Radical-induced Hetero-Nuclear Mixing and Low-field $^{13}$C Relaxation in Solid Pyruvic Acid
Source: arXiv:2202.05688 ancillary file (2022-08-01)
Supplement: Supplementary file 1 [file supplementalMaterial.pdf]

# Radical-induced Low-field $^{13}$C Relaxation and Hetero-Nuclear Mixing in Solid Pyruvic Acid: Supplemental Material

Hana Kouřilová,[1,*] Michael Jurkutat,[1,†] David Peat,[2] Karel Kouřil,[2] Alixander S. Khan,[2]
Anthony J. Horsewill,[2] James F. MacDonald,[2] John Owers-Bradley,[2] and Benno Meier[1,3,‡]

[1] *Institute of Biological Interfaces 4, Karlsruhe Institute of Technology, Germany*
[2] *School of Physics and Astronomy, University of Nottingham, Nottingham, NG7 2RD, UK*
[3] *Institute of Physical Chemistry, Karlsruhe Institute of Technology, Germany*

(Dated: July 6, 2022)

## CONTENTS

I. Samples 3
A. Sample Preparation 3
B. Sample Loading 3

II. Fast field cycling 3
A. Fast Field Cycling Apparatus 3
B. Fast Field Cycling Experiments 3
$T_1$ Measurements 3
Thermal Mixing Experiments 3

III. Spin-lattice Relaxation Data 5

IV. Thermal Mixing Data 6

V. Multi-reservoir Relaxation 8
Three reservoir relaxation 8
Carbon diffusion described by (3+1)-reservoir relaxation 8

References 9

# I. SAMPLES

## A. Sample Preparation

Neat 1-$^{13}$C-pyruvic acid was purchased from CortecNet, FR, and OX063 trityl radical was purchased from Oxford Instruments, UK. Experiments on neat pyruvic acid were carried out on a single sample, referred to as Neat PA, during a single session. Two experimental sessions were required to record data on 15 mM OX063 in 1-$^{13}$C pyruvic acid. A fresh sample was prepared for each session, and we refer to these samples as Doped PA 1 and Doped PA 2 in this manuscript. All samples were used without degassing.

## B. Sample Loading

For each experiment the corresponding solution was pipetted into either a glass tube and sealed with PTFE tape, or into a PTFE sample cup and closed using a lid with a small hole in its rotation symmetry axis to allow for the pressure equilibration. The sealed tube or the sample cup was inserted into the NMR coil. The samples were flash-frozen by immersion of the NMR probe into the cold variable temperature insert of the magnet.

# II. FAST FIELD CYCLING

## A. Fast Field Cycling Apparatus

Experiments were carried out using a fast field cycling (FFC) apparatus (Cryogenic Ltd) at the University of Nottingham, UK. The system comprises a low-inductance superconducting magnet and a fast-ramping power supply. The magnet houses a variable temperature insert (VTI). Stable temperatures in the range of 3 to 300 K and magnetic fields from 0 to 2.5 T are achieved. The magnetic field changes were performed at a rate of 4 T/s, and the absolute error of the magnetic field strength is 2 mT. A Tecmag Apollo NMR spectrometer (Tecmag, TX) with a home-written visual basic extension enables a control of the magnetic field strength from within the NMR pulse sequence. Here we used a home-built NMR probe with a solenoid tuned to a frequency of 21.6 MHz. This frequency corresponds to a resonant magnetic field of approximately 0.5 and 2 Tesla for proton and carbon spins, respectively. A more detailed description of the system has been given by Horsewill et al.[1,2].

## B. Fast Field Cycling Experiments

### *$T_1$ Measurements*

The two pulse sequences used to measure carbon relaxation are shown in Fig. S1.

For fields up to 0.2 T the equilibrium polarization signal would be too small, and so a *polarization decay* sequence that comprises an additional polarization stage (stage II) is used. In this sequence the carbon spins are first saturated to ensure reproducibility, and then polarized for 70 s at a magnetic field of 2 T. In stage III the magnetization relaxes to the new thermal equilibrium at the lower magnetic field strength. In stage IV the field is again ramped up to the resonant field and the signal is read out.

For field strengths of 0.5 T and higher a *saturation recovery* sequence was used. The carbon polarization is saturated with a train of typically 1000 8 $\mu$s $\pi/2$ pulses (stage I). Stage II in Fig. S1 is skipped and the polarization is allowed to recover for a variable time at a set field (stage III), and the magnetic field is ramped up to the detection field where the signal is read out (stage IV).

### *Thermal Mixing Experiments*

The pulse sequence used to observe thermal mixing is shown in Fig. S2. In stage I the proton magnetization reaches thermal equilibrium at the $^{13}$C resonance field of 2 T, while the carbon spins are saturated. In stage II the magnetic field is changed to the mixing field $B_{\mathrm{mix}}$ where no pulses are applied. In this period, if direct or indirect proton-carbon exchange at $B_{\mathrm{mix}}$ is possible, thermal mixing leads to a transfer of spin polarization from proton to carbon spins. In stage **III** the NMR signal is read out at the $^{13}$C resonance field of 2 T.

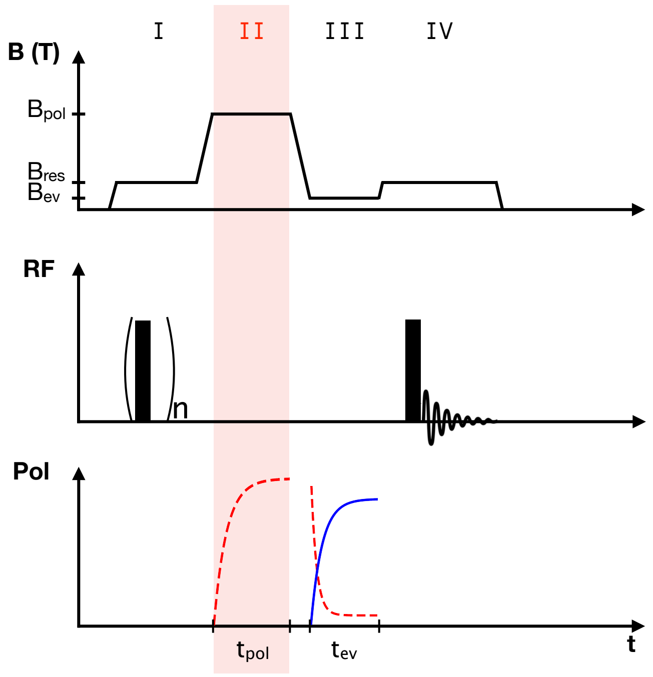


FIG. S1: Pulse sequences used for $T_1$ measurements. For fields above 0.5 T the magnetization is saturated in stage **I**. Then in stage **II** the nuclei polarize at 2 T (red dashed buildup curve). In stage **III** the field is changed to a set value and the magnetization relaxes (red dashed decay curve). In stage **IV** the NMR signal is read out. For magnetic fields of 0.5 T and higher only stages **I**, **III** and **IV** are used, i.e. stage **II** (highlighted) is dropped. For these fields the magnetization is saturated in stage **I** and recovers (blue buildup curve) in stage **III** at a set magnetic field value. In stage **IV** the NMR signal is read out. $B_{pol}$, $B_{res}$, $B_{ev}$, $t_{pol}$, $t_{ev}$ and n represent polarization magnetic field, resonance magnetic field, evolution magnetic field, polarization time, evolution time and number of saturation pulses, respectively.

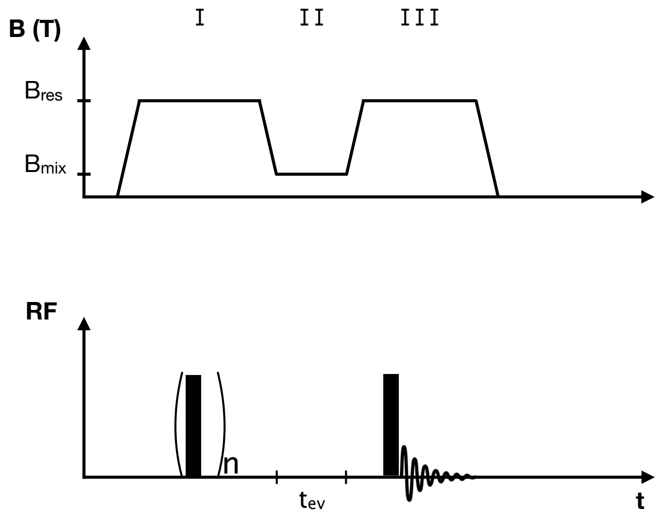


FIG. S2: Pulse sequence used for thermal mixing experiments. In stage **I** $^{13}C$ magnetization is saturated while the $^{1}H$ nuclei polarize to thermal equilibrium at the $^{13}C$ resonance field of 2 T. In stage **II** the magnetic field is changed to the mixing field and the system is left to evolve. In stage **III** the field is ramped back to the $^{13}C$ resonance field and the NMR signal is read out. Symbols $B_{res}$, $B_{mix}$, $t_{ev}$ and n represent resonance magnetic field, mixing magnetic field, evolution time and number of saturation pulses, respectively.

## III. SPIN-LATTICE RELAXATION DATA

The experimental data for the $^{13}$C $T_1$ measurements are shown in Figs. S3 and S4 together with single exponential fits.

We note that we observe ramp effects on the signal intensities. These are particularly pronounced at low evolution fields where the initial intensities ($t_{\mathrm{evo}} = 0$) appear enhanced for $^{13}$C (and diminished for $^{1}$H ). For long evolution times ($t_{\mathrm{evo}} \gg T_1$) we find signals for $^{13}$C nuclei (as well as $^{1}$H) enhanced. Numerical simulations of the interaction of both nuclear reservoirs with the electron non-Zeeman during the ramp show that the effects are qualitatively reproduced by the indirect exchange mechanism described in this manuscript, i.e. by coupling with a non-nuclear reservoir whose heat capacity is not field-dependent. However, quantitatively the calculated ramp effects including exchange with the non-Zeeman reservoir account for only about 1/3 of the observed discrepancies. Since we observe similar ramp effects in the neat sample and also for fields above 1 T, we conclude that either oxygen in our non-degassed samples is the origin or an exchange with quantized rotational states of the methyl group is responsible.

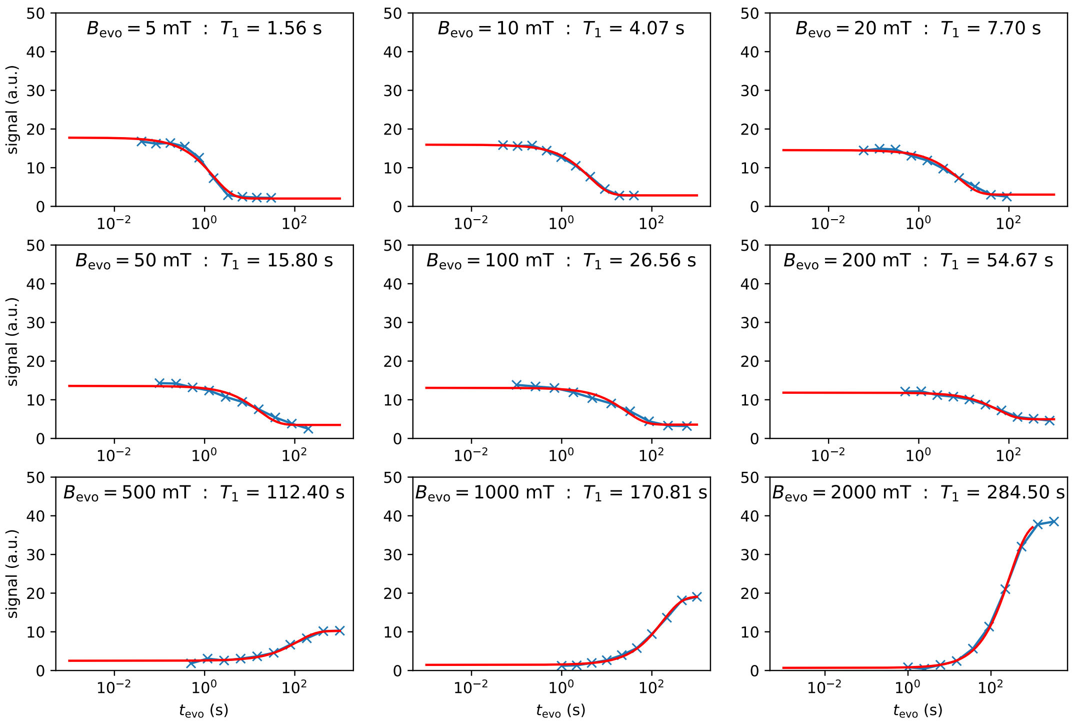


FIG. S3: $^{13}$C $T_1$ measurements on neat PA at 4 K in different fields using polarization decay up to 200 mT and saturation recovery above.

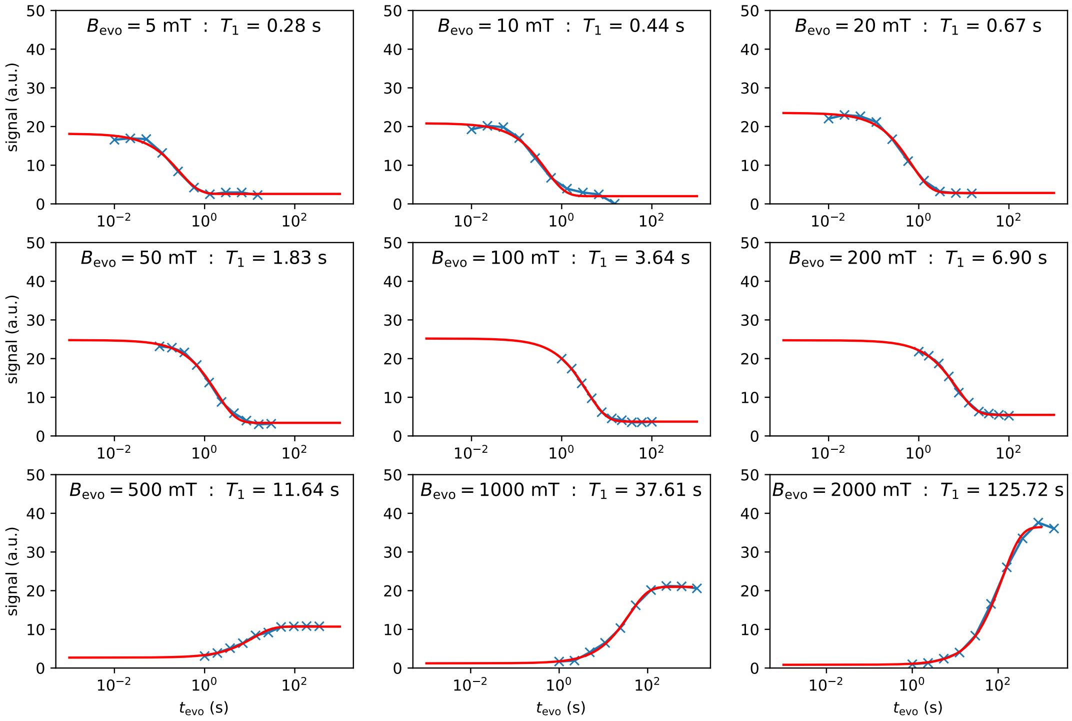


FIG. S4: $^{13}$C $T_1$ measurements on doped PA at 4 K in different fields using polarization decay up to 200 mT and saturation recovery above.

## IV. THERMAL MIXING DATA

For the experiments reported here, the equilibrium $^{13}$C signal at 2 T, cf. Fig. S4, is at the same time the maximum signal intensity that can be obtained via thermal mixing (TM), since the initially saturated carbon spins can at best be cooled down to the $^{1}$H spin temperature, which likewise equals 4.2 K at 2 T. Therefore all TM data are normalized using the $^{13}$C thermal equilibrium signal. The TM efficiency is then the ratio of the recorded $^{13}$C signal and the thermal equilibrium signal.

Fig. S5 shows a comparison of thermal mixing in pyruvic acid doped with 15 mM trityl at 3 K (first row), 4.2 K (second row), 10 K (third row), 20 K (fourth row) and in neat pyruvic acid at 4.2 K (bottom row). Note that the 4.2 K data on neat and doped pyruvic acid are also shown in the main manuscript. For each sample and temperature, the first column shows relaxation data (×) recorded with a saturation recovery sequence at the carbon detection field of 2.167 T and their fit (–). This relaxation measurement was used to scale the TM data shown in the second and third column and to calculate the TM efficiency.

For doped pyruvic acid the recorded maximum TM efficiency corresponds to approximately 28% at 3 K (at 40 mT field and 0.29 s mixing delay), 40% at 4.2 K (at 20 mT and 0.01 s), 36% at 10 K (at 30 mT and 0.054 s mixing delay) and 26% at 20 K (at 100 mT and 0.054 s mixing delay). For neat pyruvic acid, the maximum TM efficiency was 51% at 4.2 K (observed at 0 mT and 0.13 s mixing delay, as well as at 0.1 mT and 0.054 s mixing delay). As can be seen from the contour plot, our data show a local minimum in TM efficiency at 0.2 mT. This curve was reproducible. Since the absolute error of magnetic field is 2 mT, it is however likely that this data point coincides with the true zero magnetic field.

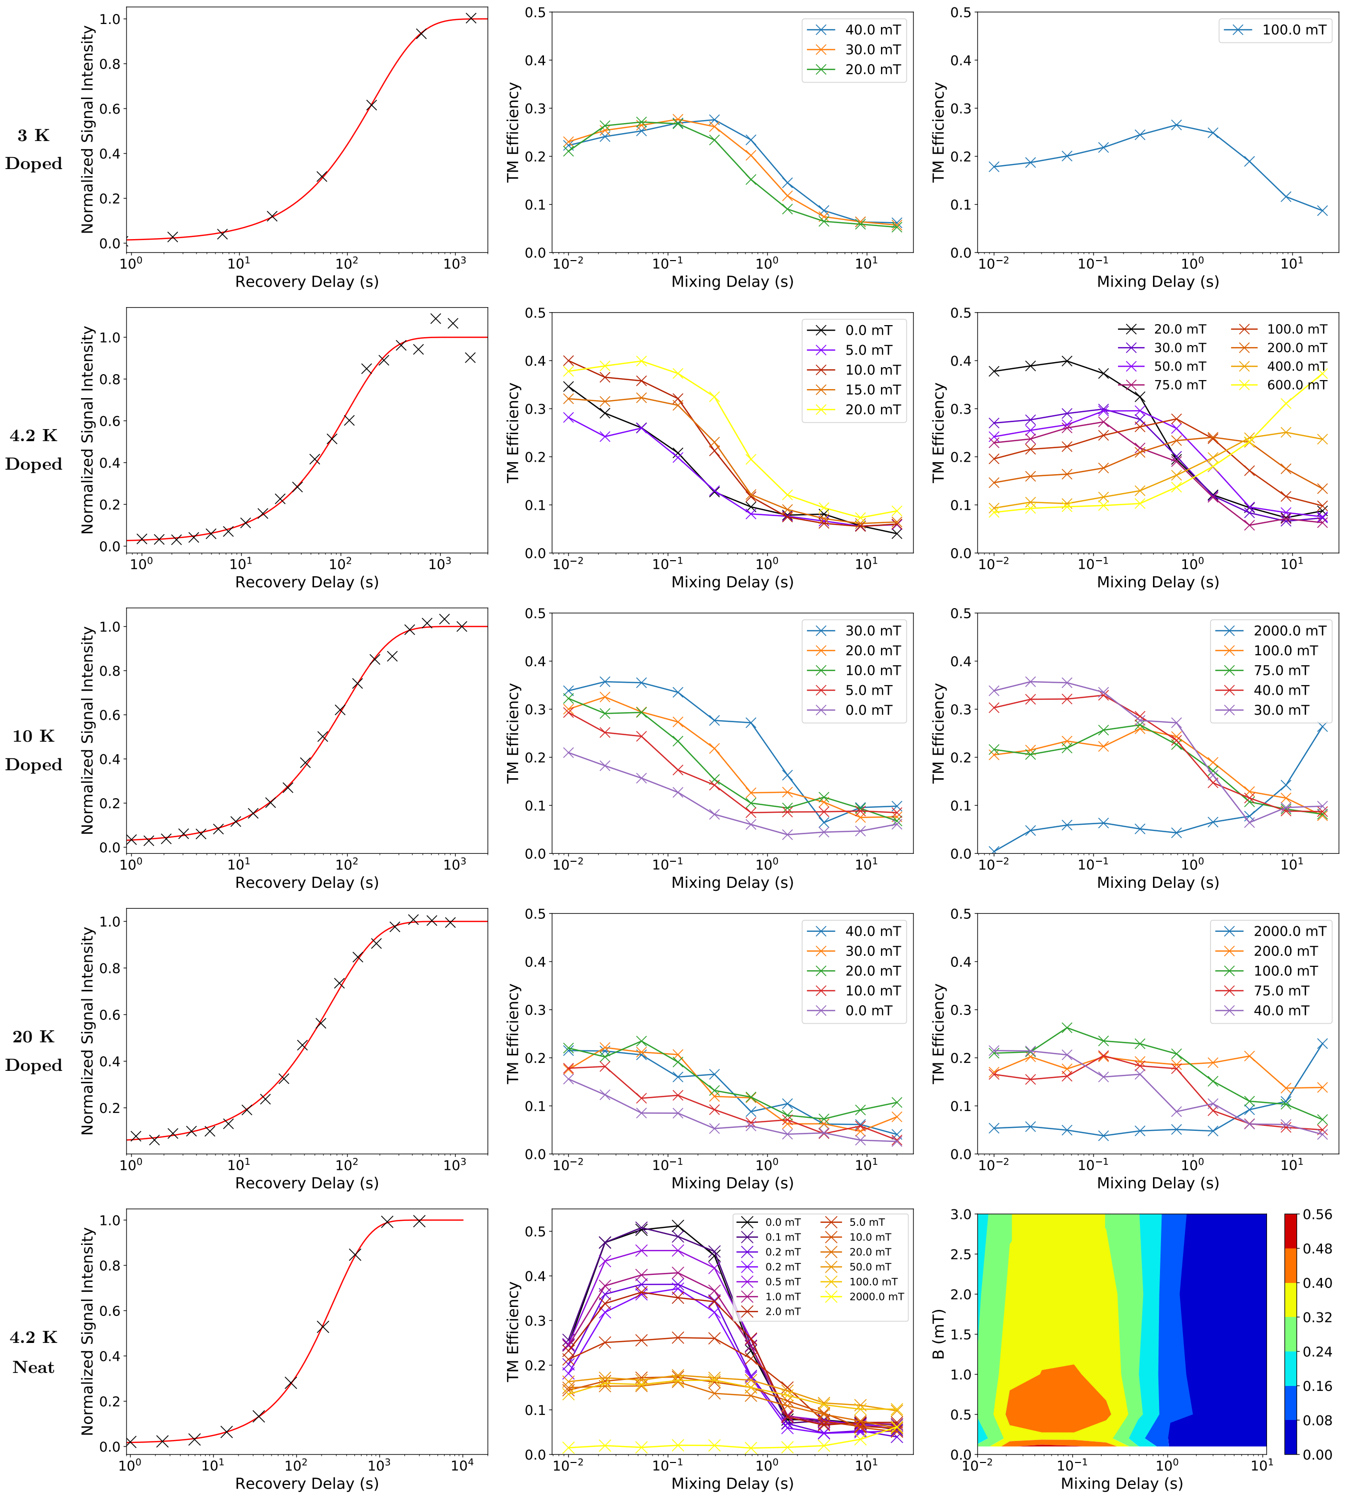


FIG. S5: Thermal mixing in doped and neat pyruvic acid at several temperatures.

## V. MULTI-RESERVOIR RELAXATION

*Three reservoir relaxation*

The heat exchange between the three reservoirs and the lattice, depicted in Fig. 2 (a) of the main manuscript, is described by set of three differential equations. These are given in matrix notation in Eq. (3) which we repeat here:

$$\frac{\partial}{\partial t}\begin{pmatrix}\beta'_{\mathrm{H}}\\ \beta'_{\mathrm{C}}\\ \beta'_{\mathrm{NZ}}\end{pmatrix} = \dot{\vec{\beta}}' = \mathcal{M}\vec{\beta}' \tag{1}$$

where the $\beta'_i = \beta_i - \beta_{\mathrm{L}}$ are the respective reservoir's difference to the inverse lattice temperature $\beta_{\mathrm{L}}$ and the relaxation matrix given by:

$$\mathcal{M} = \begin{pmatrix} -\frac{1}{\tau_{\mathrm{NZ-H}}}\frac{C_{\mathrm{NZ}}}{C_{\mathrm{H}}} - \frac{1}{\tau_{\mathrm{H-C}}}\frac{C_{\mathrm{C}}}{C_{\mathrm{H}}} - \frac{1}{T_{1,\mathrm{H}}} & \frac{1}{\tau_{\mathrm{H-C}}}\frac{C_{\mathrm{C}}}{C_{\mathrm{H}}} & \frac{1}{\tau_{\mathrm{NZ-H}}}\frac{C_{\mathrm{NZ}}}{C_{\mathrm{H}}} \\ \frac{1}{\tau_{\mathrm{H-C}}} & -\frac{1}{\tau_{\mathrm{H-C}}} - \frac{1}{\tau_{\mathrm{NZ-C}}}\frac{C_{\mathrm{NZ}}}{C_{\mathrm{C}}} - \frac{1}{T_{1,\mathrm{C}}} & \frac{1}{\tau_{\mathrm{NZ-C}}}\frac{C_{\mathrm{NZ}}}{C_{\mathrm{C}}} \\ \frac{1}{\tau_{\mathrm{NZ-H}}} & \frac{1}{\tau_{\mathrm{NZ-C}}} & -\frac{1}{\tau_{\mathrm{NZ-H}}} - \frac{1}{\tau_{\mathrm{NZ-C}}} - \frac{1}{T_{1,\mathrm{S}}} \end{pmatrix} \tag{2}$$

Here, the $C_i$ are the reservoirs' heat capacities given by Eq. (1) and (2) of the main manuscript. $\tau^{-1}_{\mathrm{NZ-H}}$ and $\tau^{-1}_{\mathrm{NZ-C}}$ are the previously calculated[?] TSF rates for proton and carbons, respectively, also displayed in Fig. 2 (b) of the main manuscript. $\tau^{-1}_{\mathrm{H-C}}$ is the direct proton-carbon exchange rate that is only non-negligible at low fields ($B < 20\,\mathrm{mT}$) where it dominates the carbon relaxation, and we find it five-fold enhanced by the addition of trityl, $\tau^{-1}_{\mathrm{H-C}} \approx 5 \cdot T^{\circ}_{1,\mathrm{C}}{}^{-1}$, in that field range. The direct nuclear spin-lattice relaxation rates are given by the measurements on neat PA, $T^{-1}_{1,\mathrm{H/C}}$, and the electron $T_{1,\mathrm{S}} \approx 5\,\mathrm{s}^{-1}$ is inferred from literature data.[3]

The Eigenvalue problem of (1) can be solved numerically for each field value by determining the eigenvalues ($\lambda_i$) and corresponding eigenvectors ($\vec{v}_i$) of the relaxation matrix $\mathcal{M}$ in (2), since all entries are derived from measurements, literature data or simulations. The resulting eigenvalues $\lambda_i$ (that we order as $0 \geq \lambda_1 \geq \lambda_2 \geq \lambda_3$ ) and corresponding eigenvectors $\vec{v}_i$ describe the three relaxation modes of the system: the slow ($\lambda_1, \vec{v}_1$), the intermediate ($\lambda_2, \vec{v}_2$) and the fast mode ($\lambda_3, \vec{v}_3$).

The solution of (1) is then

$$\vec{\beta}'(t) = \begin{pmatrix}\beta'_{\mathrm{H}}(t)\\ \beta'_{\mathrm{C}}(t)\\ \beta'_{\mathrm{NZ}}(t)\end{pmatrix} = \sum_{i=1}^{3} a_i \vec{v}_i \exp(-R_i t)\,, \tag{3}$$

where the relaxation rates $R_i = -\lambda_i$ are given by the eigenvalues and coefficients $a_i$ are determined by the initial conditions $\vec{\beta}(t=0)$.

In order to compare this three-mode relaxation to the experimentally determined single exponential decay, we can consider the combined rate at the time of measurement:

$$R_{\mathrm{H/C,comb}}(t = T^{\bullet}_{1,\mathrm{H/C}}) = -\frac{\dot{\beta}_{\mathrm{H/C}}}{\beta_{\mathrm{H/C}}}(t = T^{\bullet}_{1,\mathrm{H/C}}) = \frac{\sum_{i=1}^{3} R_i \cdot a_i \cdot v_{i,\mathrm{H/C}} \cdot \exp(-R_i t)}{\sum_{i=1}^{3} a_i \cdot v_{i,\mathrm{H/C}} \cdot \exp(-R_i t)} \tag{4}$$

The role of the different modes in the system's relaxation is less straight-forward than in the case of the two-reservoir relaxation.[?] In particular since here three, instead of one, inter-reservoir coupling rates ($\tau^{-1}_{\mathrm{H-C}}, \tau^{-1}_{\mathrm{NZ-H}}, \tau^{-1}_{\mathrm{NZ-C}}$) with differing field dependences contribute.

Nonetheless, the slow mode always describes the relaxation of the system as a whole with rate $R_1$ to the lattice temperature. All entries of the corresponding eigenvector $\vec{v}_1$ have the same sign, which signifies an overall heating or cooling of all three reservoirs with the same time constant.

The other two faster modes may also involve a net heat exchange with the lattice, but describe the internal heat exchange balancing temperature differences between the reservoirs, i.e., for both $\vec{v}_2$ and $\vec{v}_3$ one entry has an opposite sign to the other two. So these modes cool/heat one reservoir at the expense of heating/cooling the other two. Details depend on the field-dependent reservoir exchange rates and initial conditions.

*Carbon diffusion described by (3+1)-reservoir relaxation*

Only a minute part of all investigated nuclei of the substrate, in our case PA, will be close enough to radical electrons to exchange energy directly. These are referred to as *core* nuclei and their resonance frequency will also

be shifted by the radical's dipolar field, which renders them (partially) NMR-invisible. The observed NMR signal is dominated by *bulk* nuclei further away from the radical. These exchange only indirectly with the electron reservoir via spin-diffusion.[4]

The dipolar field around the radical is anisotropic and decreases continuously with distance, so there is no strict separation into core and bulk nuclei. Nonetheless it is instructive to consider and compare characteristic distances from the radical. The radius around the radicals beyond which nuclei are polarized/relaxed due to the radical only indirectly, i.e., by spin diffusion, is the so-called *diffusion boundary*, $r_{\mathrm{bo}}$. Another characteristic length is the *diffusion barrier*, $r_{\mathrm{ba}}$, which is the radius around the radical within which the resonance frequency of nuclei is changed by the nearby radicals' field to such an extent that spin diffusion to unaffected nuclei in the bulk is suppressed. Both these parameters were recently estimated to be smaller than the trityl molecule itself, $r_{\mathrm{bo}} < r_{\mathrm{ba}} < r_{\mathrm{trityl}}$.[5] So clearly, direct polarization/relaxation of the nuclear spins is limited to the radicals' immediate vicinity and spin diffusion can hinder both DNP as well as relaxation via trityl.

The exchange across the diffusion barrier was recently experimentally measured for protons in another system, and successfully modelled by two coupling reservoirs.[4] In order to incorporate carbon diffusion into the model we add a fourth reservoir by dividing the carbon reservoir into core and bulk. We scale the size of the core reservoir by a factor $\alpha \ll 1$. The bulk carbon reservoir of size $(1-\alpha)C_{\mathrm{C}}$ does not exchange energy directly with the NZ, but only with the protons, the lattice and via a spin diffusion rate $\tau_{\mathrm{C-C}}^{-1}$ with core carbons.

$$\frac{\partial \beta_{\mathrm{H}}}{\partial t} = -\frac{1}{\tau_{\mathrm{NZ-H}}}\frac{C_{\mathrm{NZ}}}{C_{\mathrm{H}}}(\beta_{\mathrm{H}}-\beta_{\mathrm{NZ}}) - \frac{1}{\tau_{\mathrm{H-C}}}\frac{\alpha\cdot C_{\mathrm{C}}}{C_{\mathrm{H}}}(\beta_{\mathrm{H}}-\beta_{\mathrm{C,co}}) - \frac{\beta_{\mathrm{H}}}{T_{1,\mathrm{H}}} - \frac{1}{\tau_{\mathrm{H-C}}}\frac{(1-\alpha)C_{\mathrm{C}}}{C_{\mathrm{H}}}(\beta_{\mathrm{H}}-\beta_{\mathrm{C,bu}}) \tag{5}$$

$$\frac{\partial \beta_{\mathrm{C,co}}}{\partial t} = +\frac{1}{\tau_{\mathrm{H-C}}}(\beta_{\mathrm{H}}-\beta_{\mathrm{C,co}}) - \frac{1}{\tau_{\mathrm{NZ-C}}}\frac{C_{\mathrm{NZ}}}{\alpha\cdot C_{\mathrm{C}}}(\beta_{\mathrm{C,co}}-\beta_{\mathrm{NZ}}) - \frac{\beta_{\mathrm{C,co}}}{T_{1,\mathrm{C}}} - \frac{1}{\tau_{\mathrm{C-C}}}\frac{1-\alpha}{\alpha}(\beta_{\mathrm{C,co}}-\beta_{\mathrm{C,bu}}) \tag{6}$$

$$\frac{\partial \beta_{\mathrm{NZ}}}{\partial t} = +\frac{1}{\tau_{\mathrm{NZ-H}}}(\beta_{\mathrm{H}}-\beta_{\mathrm{NZ}}) + \frac{1}{\tau_{\mathrm{NZ-C}}}(\beta_{\mathrm{C,co}}-\beta_{\mathrm{NZ}}) - \frac{\beta_{\mathrm{NZ}}}{T_{1,\mathrm{S}}} \tag{7}$$

$$\frac{\partial \beta_{\mathrm{C,bu}}}{\partial t} = +\frac{1}{\tau_{\mathrm{H-C}}}(\beta_{\mathrm{H}}-\beta_{\mathrm{C,bu}}) + \frac{1}{\tau_{\mathrm{C-C}}}(\beta_{\mathrm{C,co}}-\beta_{\mathrm{C,bu}}) - \frac{\beta_{\mathrm{C,bu}}}{T_{1,\mathrm{C}}} \tag{8}$$

Note that all changes from the three-reservoir description are marked in gray.

In analogy to the three-reservoir case, we can use matrix notation and the inverse temperature difference to the lattice to rewrite the set of differential equations as an eigenvalue problem:

$$\frac{\partial}{\partial t}\begin{pmatrix}\beta'_{\mathrm{H}}\\ \beta'_{\mathrm{C,co}}\\ \beta'_{\mathrm{NZ}}\\ \beta'_{\mathrm{C,bu}}\end{pmatrix} = \dot{\vec{\beta}}' = \mathcal{M}_4\vec{\beta}' \tag{9}$$

with the 4x4 relaxation matrix now given by:

$$\mathcal{M}_4 = \begin{pmatrix} -\frac{1}{\tau_{\mathrm{NZ-H}}}\frac{C_{\mathrm{NZ}}}{C_{\mathrm{H}}} - \frac{1}{\tau_{\mathrm{H-C}}}\frac{C_{\mathrm{C}}}{C_{\mathrm{H}}} - \frac{1}{T_{1,\mathrm{H}}} & \frac{1}{\tau_{\mathrm{H-C}}}\frac{C_{\mathrm{C}}\cdot\alpha}{C_{\mathrm{H}}} & \frac{1}{\tau_{\mathrm{NZ-H}}}\frac{C_{\mathrm{NZ}}}{C_{\mathrm{H}}} & \frac{1}{\tau_{\mathrm{H-C}}}\frac{C_{\mathrm{C}}\cdot(1-\alpha)}{C_{\mathrm{H}}} \\ \frac{1}{\tau_{\mathrm{H-C}}} & -\frac{1}{\tau_{\mathrm{H-C}}} - \frac{1}{\tau_{\mathrm{NZ-C}}}\frac{C_{\mathrm{NZ}}}{C_{\mathrm{C}}\cdot\alpha} - \frac{1}{T_{1,\mathrm{C}}} - \frac{1}{\tau_{\mathrm{C-C}}}\frac{(1-\alpha)}{\alpha} & \frac{1}{\tau_{\mathrm{NZ-C}}}\frac{C_{\mathrm{NZ}}}{C_{\mathrm{C}}\cdot\alpha} & \frac{1}{\tau_{\mathrm{C-C}}}\frac{(1-\alpha)}{\alpha} \\ \frac{1}{\tau_{\mathrm{NZ-H}}} & \frac{1}{\tau_{\mathrm{NZ-C}}} & -\frac{1}{\tau_{\mathrm{NZ-H}}} - \frac{1}{\tau_{\mathrm{NZ-C}}} - \frac{1}{T_{1,\mathrm{S}}} & 0 \\ \frac{1}{\tau_{\mathrm{H-C}}} & \frac{1}{\tau_{\mathrm{C-C}}} & 0 & -\frac{1}{\tau_{\mathrm{H-C}}} - \frac{1}{\tau_{\mathrm{C-C}}} - \frac{1}{T_{1,\mathrm{C}}} \end{pmatrix} \tag{10}$$

The solution is analogous to that for the three reservoir systems described above. The expected observable single-exponential carbon relaxation rate $R'_{\mathrm{C,comb}}$ is given by a weighted average of the core and bulk carbon nuclei. However, since the core nuclei are few ($\alpha \gtrsim 0$) and it is uncertain to what extent they are NMR-visible, the observed $R'_{\mathrm{C,comb}}$ is corresponds to that of the bulk carbon nuclei:

$$R'_{\mathrm{C,comb}}(t=T^{\bullet}_{1,\mathrm{C}}) = \alpha\cdot R_{\mathrm{C,co,comb}}(t=T^{\bullet}_{1,\mathrm{C}}) + (1-\alpha)\cdot R_{\mathrm{C,bu,comb}}(t=T^{\bullet}_{1,\mathrm{C}}) \underset{\alpha\approx 0}{\approx} R_{\mathrm{C,bu,comb}}(t=T^{\bullet}_{1,\mathrm{C}}) \tag{11}$$

We find that a field-dependent carbon core-bulk diffusion time constant $\tau_{\mathrm{C-C}} = B\cdot 33\,\mathrm{s/T}$ describes the experimental data well. Note that the resulting carbon rate is fairly insensitive to the value of $\alpha \ll 1$, and that in the employed reservoir description the core-bulk diffusion rate $\tau_{\mathrm{C-C}}^{-1}$ could result from either limited core-bulk exchange (across the diffusion barrier) or from limited carbon diffusion in the bulk.

* hana.kourilova@kit.edu

[†] michael.jurkutat@kit.edu
[‡] benno.meier@kit.edu

[1] A. J. Horsewill and Q. Xue, Phys. Chem. Chem. Phys. **4**, 5475 (2002).
[2] D. T. Peat, M. L. Hirsch, D. G. Gadian, A. J. Horsewill, J. R. Owers-Bradley, and J. G. Kempf, Physical Chemistry Chemical Physics **18**, 19173 (2016).
[3] L. Lumata, Z. Kovacs, A. D. Sherry, C. Malloy, S. Hill, J. van Tol, L. Yu, L. Song, and M. E. Merritt, Phys. Chem. Chem. Phys. **15**, 9800 (2013).
[4] Q. Stern, S. F. Cousin, F. Mentink-Vigier, A. C. Pinon, S. J. Elliott, O. Cala, and S. Jannin, Science Advances **7**, nil (2021).
[5] W. Wenckebach, A. Capozzi, S. Patel, and J. Ardenkjær-Larsen, Journal of Magnetic Resonance **327**, 106982 (2021).
